# Supplementary material for: TBD: Benchmarking and Analyzing Deep Neural Network Training
Source: arXiv:1803.06905 source file (2018-04-14)
Supplement: Supplementary file 1 [file appendix.tex]

\section{appendix}

\begin{figure}
    \centering
    \includegraphics[width=0.48\textwidth]{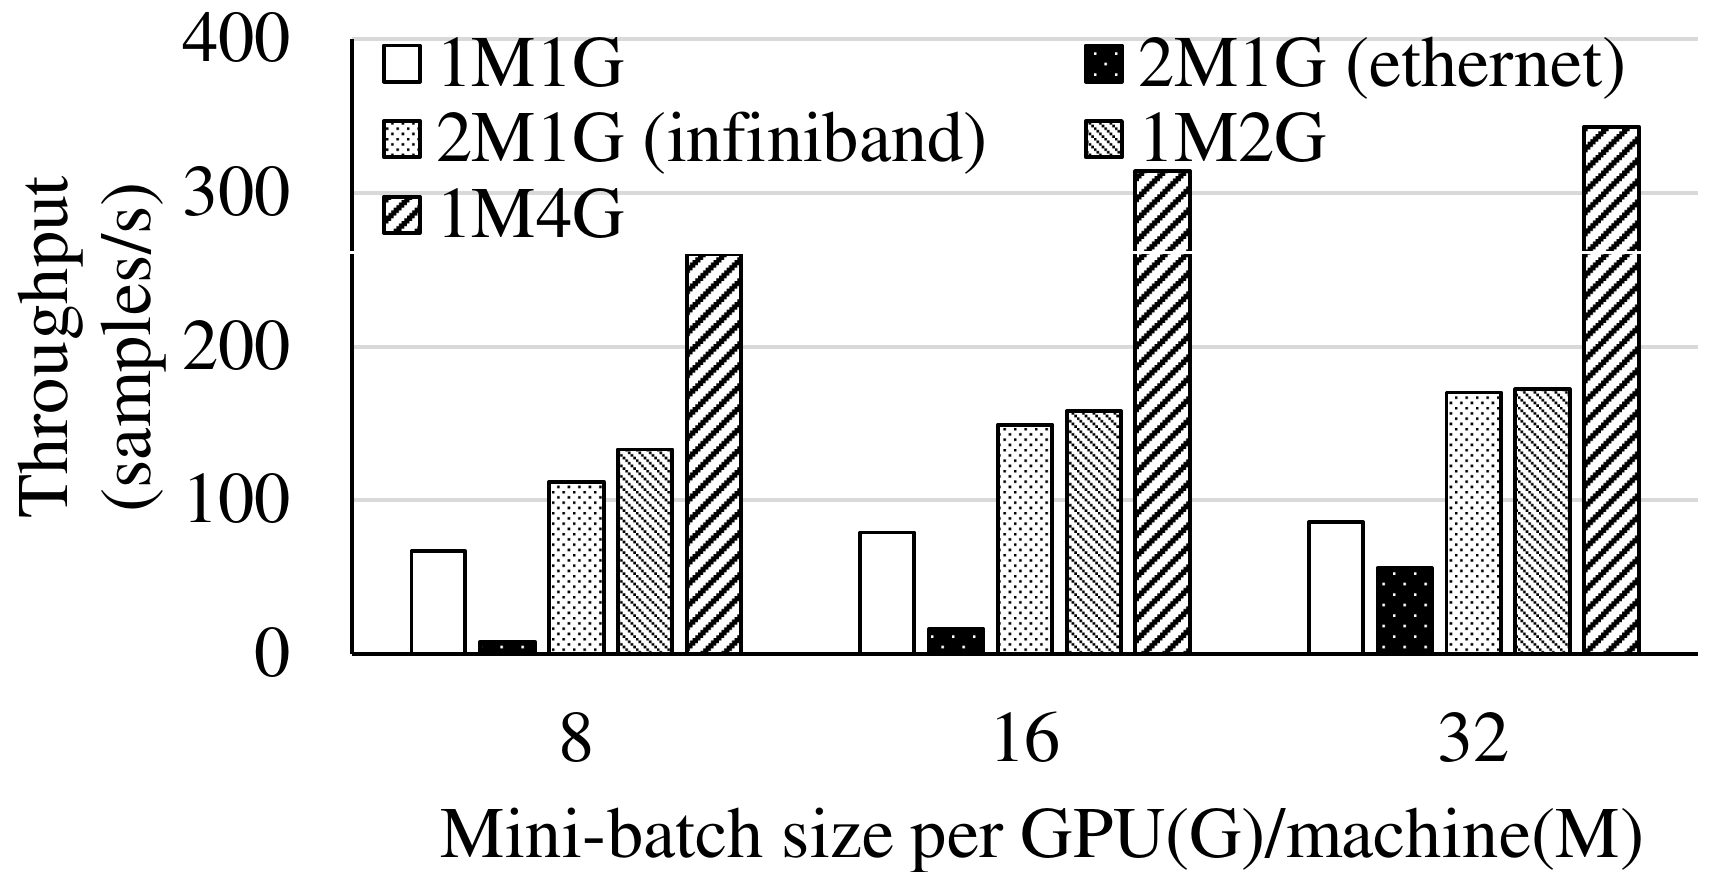}
    \caption{ResNet-50 on MXNet with multiple GPUs/machines.}
    \label{fig:distributed}
\end{figure}
